# Supplementary material for: PaCo: Preconditions Attributed to Commonsense Knowledge
Source: arXiv:2104.08712 source file (2023-08-13)
Supplement: Supplementary file 1 [file AppendixDatasheet.tex]

\TODO{Write this document}
\paragraph{What do the instances that comprise the dataset represent?}
(e.g.,documents, photos, people, countries)
Are there multiple types of instances (e.g., movies, users, and ratings; people and interactions between them; nodes and edges)?
Please provide a description.
\paragraph{How many instances are there in total?}
 (of each type, if appropriate)

\paragraph{Does the dataset contain all possible instances or is it a sample (not necessarily random) of instances from a larger set?}
If the dataset is a sample, then what is the larger set?
Is the sample representative of the larger set (e.g., geographic coverage)? If so, please describe how
this representativeness was validated/verified.
If it is not representative of the larger set, please describe why not (e.g., to cover a more diverse range of instances, because instances were withheld or unavailable).
\paragraph{What data does each instance consist of? “Raw” data (e.g., unprocessed text or images) or features?}
In either case, please provide a description.
\paragraph{Is there a label or target associated with each instance?}
If so, please provide a description.
\paragraph{Is any information missing from individual instances?}
If so, please provide a description, explaining why this information is missing (e.g.,
because it was unavailable).
This does not include intentionally removed
information, but might include, e.g., redacted text.
\paragraph{Are relationships between individual instances made explicit
(e.g., users’ movie ratings, social network links)?}
If so, please describe how these relationships are made explicit.
\paragraph{Are there recommended data splits (e.g., training, development/validation, testing)?}
If so, please provide a description of these splits, explaining
the rationale behind them.
\paragraph{Are there any errors, sources of noise, or redundancies in the
dataset?}
If so, please provide a description.
\paragraph{Is the dataset self-contained, or does it link to or otherwise rely on external resources (e.g., websites, tweets, other datasets)?}
If it links to or relies on external resources, a) are there guarantees that they will
exist, and remain constant, over time; b) are there official archival versions
of the complete dataset (i.e., including the external resources as they
existed at the time the dataset was created); c) are there any restrictions
(e.g., licenses, fees) associated with any of the external resources that
might apply to a future user? Please provide descriptions of all external
resources and any restrictions associated with them, as well as links or
other access points, as appropriate.

\paragraph{Does the dataset contain data that might be considered confidential (e.g., data that is protected by legal privilege or by doctorpatient confidentiality, data that includes the content of individuals’ non-public communications)?}
If so, please provide a description.
\paragraph{Does the dataset contain data that, if viewed directly, might be offensive, insulting, threatening, or might otherwise cause anxiety?}
If so, please describe why.
\paragraph{Does the dataset relate to people?}
If not, you may skip the remaining
questions in this section.
\paragraph{Does the dataset identify any subpopulations (e.g., by age, gender)?}
If so, please describe how these subpopulations are identified and provide a description of their respective distributions within the dataset.
\paragraph{Is it possible to identify individuals (i.e., one or more natural persons), either directly or indirectly (i.e., in combination with other
data) from the dataset?}
If so, please describe how.
\paragraph{Does the dataset contain data that might be considered sensitive
in any way?}
(e.g., data that reveals racial or ethnic origins, sexual
orientations, religious beliefs, political opinions or union memberships, or locations; financial or health data; biometric or genetic data; forms of government identification, such as social security numbers; criminal history)? If so, please provide a description.
\paragraph{Any other comments?}
